# Supplementary material for: On the Luttinger-Ward functional and the convergence of skeleton diagrammatic series expansion of the self-energy for Hubbard-like models
Source: arXiv:2108.10903 ancillary file (2021-08-24)
Supplement: Supplementary file 1 [file LuttingerWardSkeleton.pdf]

In[1]:=

```
(* Luttinger-Ward-Skeleton |
The following codes have been largely included as references of the publication
On the Luttinger-Ward functional and the convergence of skeleton
diagrammatic series expansion of the self-energy for Hubbard-like models,
by Behnam Farid -
24 August 2021. The codes below for Equiv and Verify are presented in Sec. D
.4 [Symbolic computation] of appendix D of the mentioned publication. This
notebook will be published (as an Ancillary file) along with the above-
mentioned text at arXiv. In due course it will also be published
at Notebook Archive of Wolfram Notebook Technology [1]. |
Copyright © 2021 by Behnam Farid. All programs,
algorithms, and methods presented here,
as well as in the publication indicated above,
are intellectual property of the author. Any commercial use of these without
his written permission is strictly prohibited. All academic and non-
commercial uses of the codes in this notebook, or modifications thereof,
must appropriately cite both this work and the above-mentioned publication. |
Do not modify this heading. *)
```

In[2]:=

```
(* Reference *)
```

In[3]:= (\* [1] \*) URL["https://www.notebookarchive.org/search?q=Behnam Farid"]

Out[3]:= URL[<https://www.notebookarchive.org/search?q=Behnam Farid> >>]

In[4]:=

```
(* End of Reference *)
```

In[5]:= (\* When using this notebook for the first time,  
use preferably *Evaluate Notebook* [under Evaluation] \*)In[6]:= (\* Included as references of the above-mentioned publication -  
reference numbers [of the arXiv publication] are given inside the square brackets \*)

In[7]:= (\* Ref. [51] \*)

In[8]:= ClearAll[f, S, j];  
f[z\_, n\_] := -z / (ħ (1 + Sum["G<sub>∞</sub>"<sub>j+1</sub> / z<sup>j</sup>, {j, 1, n + 2}] / ħ);  
S[j\_] := SeriesCoefficient[f[z, j], {z, Infinity, j}];

In[9]:= j = 3 (\* To be varied\*);

In[10]:= Print[Subscript[Σ<sub>∞</sub>, j], " = ", S[j]]

$$\Sigma_{\infty 3} = \frac{-G_{\infty 2}^4 + 3 \hbar G_{\infty 2}^2 G_{\infty 3}^2 - \hbar^2 G_{\infty 3}^2 - 2 \hbar^2 G_{\infty 2} G_{\infty 4} + \hbar^3 G_{\infty 5}}{\hbar^5}$$

In[11]:= (\* Ref. [71] \*)

```

In[12]:= ClearAll[S, m, p, q, PA];
S[z_, e_, m_] := Sum[(1 + (-1)^nu) (e / z)^nu, {nu, 0, m}] / (2 z);
m = 2 (*To be varied*);
p = Floor[m / 2];
q = p + 1;
Print["The [p/q] = ", "[", p, "/", q, "] Padé approximant of G(z,ε):"];
PA = PadeApproximant[S[z, ε, m], {z, Infinity, {p, q}}];
Print["G(z,ε) = ", Apart[PA, z]]

The [p/q] = [1/2] Padé approximant of G(z,ε):


$$G(z, \epsilon) = \frac{1}{2(z - \epsilon)} + \frac{1}{2(z + \epsilon)}$$


In[13]:= (* Ref. [87] *)

In[14]:= ClearAll[ei, Theta, Hat, f0, f1, Resj, Minim, A];
ei[i_, mu_, Delta_, M_] := mu + Delta (2 (i - 1 / 2) / M - 1) / 2;
Theta[x_, eta_] := (1 + Tanh[x / eta]) / 2;
Hat[x_, eta_, d_] := Theta[x + d / 2, eta] - Theta[x - d / 2, eta];
f0[e0_, xx_, jx_] := f0[e0, xx, jx] = ((e0 + xx)^jx - (e0 - xx)^jx) / jx;
f1[e0_, xx_, jx_] :=
  f1[e0, xx, jx] = NIntegrate[SetPrecision[Hat[e - e0, xx, 2 xx] e^(jx - 1), Infinity],
    {e, -Infinity, Infinity}, WorkingPrecision -> 64, MaxRecursion -> 1000];
Resj[j_, U_, mu_, eta_, Delta_, M_, iex_, a_] := Module[
  (*Square of the j-th residual error, specific to the `Hubbard atom'. For iex =
  0 moments are calculated inexactly (they are exact for eta = 0^+),
  and for iex ≠ 0 they are calculated numerically `exactly';
  the latter calculations are time-consuming. For increasing values of M the
  absolute difference between any exactly-calculated moment and its inexactly-
  calculated counterpart diminishes. *) {x, p, r, Ux, i}, x = Delta / (2 M);
  Ux = If[Mod[j, 2] == 0, 0, U];
  p = If[iex == 0, Sum[a[i] × f0[ei[i, mu, Delta, M], x, j], {i, 1, M}],
    Sum[a[i] × f1[ei[i, mu, Delta, M], x, j], {i, 1, M}]];
  r = If[j == 1, (p - 1)^2, (p - (Ux / 2)^(j - 1))^2];
  r];
Minim[mn_, U_, mu_, eta_, Delta_, M_, iex_] := Module[(*Determines the variational
  constants {alpha_j | j = 1, 2, ..., M} through minimising Sum_{j=1}^{mn} Resj.*)
  {ar, br, alpha, arx, j}, arx = Array[ar, M, {1, M}];
  br = NMinimize[{Sum[Resj[j, U, mu, eta, Delta, M, iex, ar], {j, 1, mn}],
    arx ∈ NonNegativeReals}, arx, MaxIterations -> 2000];
  Print["Residual Error: ", Sqrt[br[[1]]]];
  Do[alpha[j] = br[[2, j, 2]], {j, 1, M}];
  alpha]; A[e_, mu_, eta_, Delta_, M_, a_] :=
Module[(*Single-particle spectral function, specific to the `Hubbard atom'.*)
  {p, i}, p = Sum[a[i] × Hat[e - ei[i, mu, Delta, M], eta, Delta / M], {i, 1, M}];
  p];

```

```

In[15]:= ClearAll[U, mu, M, Delta, mn, iex, eta, alpha, gr];
U = 1 (*To be varied*);
mu = 0 (*To be varied*);
M = 100 (*To be varied*);
Delta = 2 U (*To be varied*);
mn = 5 (*Number of moments - To be varied*);
iex = 0 (*0 = Approximate; 1 = `Exact' - To be varied*);
eta = Delta / (2 M);
alpha = Minim[mn, U, mu, eta, Delta, M, iex];
gr = Plot[{A[e, mu, eta, Delta, M, alpha]},
  {e, -Delta / 2, Delta / 2}, PlotRange -> All, AxesOrigin -> {mu, 0}]

```

Residual Error: 0.000159432

Out[15]=

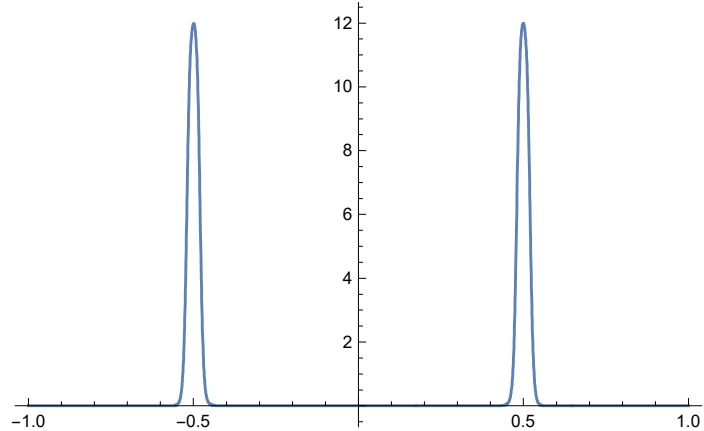

```

In[16]:= (* Test *)

```

```

In[17]:= ClearAll[pg, mr, wp, s0, s1, s2];

```

```

In[18]:= pg = 8 (*Precision Goal*);
mr = 1000 (*Max Recursion*);
wp = 32 (*Working Precision*);

In[19]:= s0 = NIntegrate[SetPrecision[A[e, mu, eta, Delta, M, alpha], Infinity],
  {e, -Delta / 2, Delta / 2}, MaxRecursion -> mr, WorkingPrecision -> wp,
  PrecisionGoal -> pg] (* 0th-order moment - Exact: 1 *);
Print["=> The 0th-order moment of A(ε): ", Style[N[s0, pg], Red],
  ". Exact: ", Style[1, Darker[Green]]]

```

=> The 0th-order moment of A(ε): 1.0000083. Exact: 1

```

In[20]:= s1 = NIntegrate[SetPrecision[e A[e, mu, eta, Delta, M, alpha], Infinity],
  {e, -Delta / 2, Delta / 2}, MaxRecursion -> mr, WorkingPrecision -> wp,
  PrecisionGoal -> pg] (* 1st-order moment - Exact: 0 *);
Print["=> The 1st-order moment of A(ε): ", Style[N[s1, pg], Red],
  ". Exact: ", Style[0, Darker[Green]]]

```

=> The 1st-order moment of A(ε): -1.6878666 × 10<sup>-15</sup>. Exact: 0

```

In[21]:= s2 = NIntegrate[SetPrecision[e^2 A[e, mu, eta, Delta, M, alpha], Infinity],
  {e, -Delta / 2, Delta / 2}, PrecisionGoal → pg, MaxRecursion → mr, WorkingPrecision → wp,
  PrecisionGoal → pg] (* 2nd-order moment - Exact: (U/2)^2 *);
Print["⇒ The 2nd-order moment of A(ε): ", Style[N[s2, pg], Red],
  ". Exact: ", Style[(U / 2.0)^2, Darker[Green]]]
⇒ The 2nd-order moment of A(ε): 0.25001045. Exact: 0.25

In[22]:= (* Ref. [106] *)

In[23]:= (* To calculate P∞j in terms of {χ∞i | i=2, ..., j} *)

In[24]:= ClearAll[Pinf, j];
Pinf[n_] := Module[{c, j, f, g}, c[j_] := If[Mod[j, 2] == 1, 0, "χ∞"j];
  f[j_] := "f"j;
  f[1] = 0;
  Do[f[j] = "v" (c[j] - Sum[c[j1] × f[j - j1], {j1, 1, j - 1}]), {j, 2, n}];
  g = (Expand[f[n] / "v"] /. Plus → (Defer[+###] ~Reverse~ {2} &));
  g];

In[25]:= j = 6 (*To be varied*); Print[Subscript[P∞, j], " = ", Pinf[j]]
P∞6 = χ∞6 - 2 v χ∞2 χ∞4 + v2 χ∞23

In[26]:= (* Alternative - Direct, non-recursive *)

In[27]:= ClearAll[Pinf, j];
Pinf[n_] := Module[{Chi, P, z, g},
  Chi[z_, nx_] := Sum[Subscript["χ∞", 2 j] / z^(2 j), {j, 1, Floor[nx / 2]}];
  P[z_, nx_] := Normal[Series[Chi[z, nx] / (1 + "v" Chi[z, nx]), {z, Infinity, nx}]];
  g = Coefficient[P[z, n], 1 / z, n] /. Plus → (Defer[+###] ~Reverse~ {2} &);
  g];

In[28]:= j = 6 (*To be varied*); Print[Subscript[P∞, j], " = ", Pinf[j]]
P∞6 = χ∞6 - 2 v χ∞2 χ∞4 + v2 χ∞23

In[29]:= (* To calculate χ∞j in terms of {P∞i | i=2, ..., j} *)

In[30]:= ClearAll[Chiinf, j];
Chiinf[n_] := Module[{P, Chi, z, g},
  P[z_, nx_] := Sum[Subscript["P∞", 2 j] / z^(2 j), {j, 1, Floor[nx / 2]}];
  Chi[z_, nx_] := Normal[Series[P[z, nx] / (1 - "v" P[z, nx]), {z, Infinity, nx}]];
  g = Coefficient[Chi[z, n], 1 / z, n] /. Plus → (Defer[+###] ~Reverse~ {2} &);
  g];

In[31]:= j = 6 (*To be varied*); Print[Subscript[χ∞, j], " = ", Chiinf[j]]
χ∞6 = P∞6 + 2 v P∞2 P∞4 + v2 P∞23

In[32]:= (* Ref. [122] *)

In[33]:= (* The equation/page numbers below followed by `(A)' correspond to
  `The Classical Moment Problem and some related questions in analysis',
  by N. I. Akhiezer (Oliver & Boyd, Edinburgh, 1965) *)

```

```

In[34]:= ClearAll[Hm, Dk, Mk, Pn, Qn, Betaj, LO, InProd, z];
Hm[m_] := Module[
  (*The (m+1) × (m+1) Hankel moment matrix - p. 1 (A)*) {k, j, T1, T2, hm}, k = m + 1;
  T1 = Table[sj, {j, 0, k - 1}];
  T2 = Table[sj, {j, k - 1, 2 k - 2}];
  hm = HankelMatrix[T1, T2];
  hm];
Dk[k_] := Module[(*The determinant Dk of the (k+1) × (k+1) Hankel moment matrix -
  p. 1 (A)*) {hm, d}, hm = Hm[k];
  d = Det[hm];
  d];
Mk[n_, z_] := Module[(*The (n+1) × (n+1) matrix whose determinant
  up to normalisation determines the polynomial Pn(z) - Eq. [1.4],
  p. 3 (A)*) {j, T1, T2, T3, Hk, A}, T1 = Table[sj, {j, 0, n - 1}];
  T2 = Table[sj, {j, n - 1, 2 n - 1}];
  T3 = Table[z^j, {j, 0, n}];
  Hk = HankelMatrix[T1, T2];
  A = Append[Hk, T3];
  A];
Pn[n_, z_] := Module[(*The nth-order polynomial Pn(z);
  P0(z) = 1/Sqrt[s0] - Eq. [1.4], p. 3 (A)*) {P},
  P = If[n == 0, 1 / Sqrt[s0], Det[Mk[n, z]] / Sqrt[Dk[n - 1] × Dk[n]]] (* Substitute
    the 1/Sqrt[s0] by 1 in order to observe the consequence(s) of P0(z) = 1 *);
  P];
Qn[n_, z_, P_] := Module[(*The (n-1)th-
  order polynomial Qn(z) associated with the nth-order polynomial Pn(z),
  making use of the expression in Eq. (B.89) of the publication - Eq. [1.14],
  p. 8 (A)*) {qq, pmp, qx, x}, qq[p_, np_] := Module[{q, px, j}, ClearAll[s, x];
  px = 0;
  Do[px = px + Coefficient[p, x, j] × Subscript[s, j], {j, 0, np}];
  px];
  pmp = (P[n, z] - P[n, x]) / (z - x);
  qx = Simplify[qq[pmp, n - 1] / Subscript[s, 0]];
  qx];
Betaj[j_] :=
  If[j == 1, Simplify[Dk[1] / Dk[0]^2], Simplify[Dk[j - 2] × Dk[j] / Dk[j - 1]^2]] (*βj*) ;
LO[n_, z_] := Simplify[Qn[n, z, Pn] × Pn[n - 1, z] - Qn[n - 1, z, Pn] × Pn[n, z],
  Assumptions → {s0 > 0}] (*Liouville-Ostrogradskii*);
InProd[m_, n_] := Module[(*Returns the inner product of Pm(z) and Pn(z), using the
  measure to which the positive sequence {s0, s1, s2, ...} corresponds. Here m,
  n ∈ {0, 1, 2, ...}*) {qq, PmPn, qx}, qq[p_, np_] := Module[{q, px, j}, ClearAll[s, z];
  px = 0;
  Do[px = px + Coefficient[p, z, j] × Subscript[s, j], {j, 0, np}];
  px];
  PmPn = Normal[Series[Pn[m, z] × Pn[n, z], {z, 0, m + n}]];
  qx = Simplify[qq[PmPn, n + m]];
  qx];

```

```

In[35]:= (* For determining  $P_n(z)$  and  $Q_n(z)$  by solving the relevant three-
term recurrence relation subject to appropriate initial conditions -
 $\{P_j(z) \mid j = 0, 1, 2, \dots\}$  normalised to unity. *)

In[36]:= ClearAll[rec, k, y, PQn, PnRec, QnRec, LORec];
rec = Sqrt[Subscript[ $\beta$ , k]] y[k - 1] +
Subscript[ $\alpha$ , k + 1]  $\times$  y[k] + Sqrt[Subscript[ $\beta$ , k + 1]] y[k + 1] == z y[k];
PQn[n_, {PQ0_, PQ1_}] := First[RecurrenceTable[
rec && y[0] == PQ0 && y[1] == PQ1, y, {k, n, n}]];
PnRec[n_, z_] := PQn[n, {1 / Sqrt[Subscript[s, 0]],
(z - Subscript[ $\alpha$ , 1]) / Sqrt[Subscript[s, 0]  $\times$  Subscript[ $\beta$ , 1]]}] (* $P_n(z)$ *);
QnRec[n_, z_] := PQn[n, {0, 1 / Sqrt[Subscript[s, 0]  $\times$  Subscript[ $\beta$ , 1]]}] (* $Q_n(z)$ *);
LORec[n_, z_] := Simplify[PnRec[n - 1, z]  $\times$  QnRec[n, z] - PnRec[n, z]  $\times$  QnRec[n - 1, z],
Assumptions  $\rightarrow$  { $s_0 > 0$ }] (*Liouville-Ostrogradskii*);

In[37]:= ClearAll[n, n1, Px, Qx, Qy];
n = 2 (*To be varied*);
Print[Subscript[H, n], " = ", MatrixForm[Hm[n]]]


$$\mathbb{H}_2 = \begin{pmatrix} s_0 & s_1 & s_2 \\ s_1 & s_2 & s_3 \\ s_2 & s_3 & s_4 \end{pmatrix}$$


In[38]:= Print["The principal minors of the above Hankel moment matrix, ",
Subscript[H, n], ":"];
Do[Print[Subscript[D, m], " = ", Dk[m]], {m, 0, n}]
The principal minors of the above Hankel moment matrix,  $\mathbb{H}_2$ :

$$D_0 = s_0$$


$$D_1 = -s_1^2 + s_0 s_2$$


$$D_2 = -s_2^3 + 2 s_1 s_2 s_3 - s_0 s_3^2 - s_1^2 s_4 + s_0 s_2 s_4$$


In[39]:= Print[Subscript[M, n], " = ", MatrixForm[Mk[n, z]]]


$$\mathbb{M}_2 = \begin{pmatrix} s_0 & s_1 & s_2 \\ s_1 & s_2 & s_3 \\ 1 & z & z^2 \end{pmatrix}$$


In[40]:= Print[Subscript[P, n], "(z) = ",
Simplify[Pn[n, z], Assumptions  $\rightarrow$  {Subscript[s, 0] > 0}]]

$$P_2(z) = \frac{-z^2 s_1^2 - s_2^2 + z s_0 (z s_2 - s_3) + s_1 (z s_2 + s_3)}{\sqrt{(s_1^2 - s_0 s_2) (s_2^3 + s_0 s_3^2 + s_1^2 s_4 - s_2 (2 s_1 s_3 + s_0 s_4))}}$$


In[41]:= Print[Subscript[Q, n], "(z) = ",
Simplify[Qn[n, z, Pn], Assumptions  $\rightarrow$  {Subscript[s, 0] > 0}]]

$$Q_2(z) = \frac{-s_1^3 + s_0 s_1 (-z s_1 + 2 s_2) + s_0^2 (z s_2 - s_3)}{s_0 \sqrt{(s_1^2 - s_0 s_2) (s_2^3 + s_0 s_3^2 + s_1^2 s_4 - s_2 (2 s_1 s_3 + s_0 s_4))}}$$


```

```

In[42]:= Clear[nm, k];
nm = 2 n (*To be varied*);
Print["The inner products  $\langle P_i, P_j \rangle$  for  $i \in \{0, 1, \dots, nm\}$ ,
", j  $\in \{0, \dots, i\}$  (Total number: ", (nm + 1) (nm + 2) / 2, "):"];
k = 0;
Do[k = k + 1;
  Print["<", Subscript[P, i], ", ", Subscript[P, j],
    "> = ", InProd[i, j], " ..... (", k, ")"], {i, 0, nm}, {j, 0, i}];
Clear[k];

The inner products  $\langle P_i, P_j \rangle$  for  $i \in \{0, 1, \dots, 4\}$ ,  $j \in \{0, \dots, i\}$  (Total number: 15):

<P0, P0> = 1 ..... (1)
<P1, P0> = 0 ..... (2)
<P1, P1> = 1 ..... (3)
<P2, P0> = 0 ..... (4)
<P2, P1> = 0 ..... (5)
<P2, P2> = 1 ..... (6)
<P3, P0> = 0 ..... (7)
<P3, P1> = 0 ..... (8)
<P3, P2> = 0 ..... (9)
<P3, P3> = 1 ..... (10)
<P4, P0> = 0 ..... (11)
<P4, P1> = 0 ..... (12)
<P4, P2> = 0 ..... (13)
<P4, P3> = 0 ..... (14)
<P4, P4> = 1 ..... (15)

```

```

In[43]:= Print["Deduced from the leading principal minors of the
  Hankel moment matrix [compare with the expression(s) below]:"];
Do[Print[Subscript[β, j], " = ", Beta[j]], {j, 1, n}];
Print["Deduced from the Liouville–Ostrogradskii
  formula [compare with the expression(s) above]:"];
Do[Print[Subscript[β, j], " = ", Simplify[1 / (Subscript[s, 0] × LO[j, z]) ^ 2,
  Assumptions -> Subscript[s, 0] > 0]], {j, 1, n}]

```

Deduced from the leading principal minors of  
the Hankel moment matrix [compare with the expression(s) below]:

$$\beta_1 = \frac{-s_1^2 + s_0 s_2}{s_0^2}$$

$$\beta_2 = \frac{s_0 (-s_2^3 - s_0 s_3^2 - s_1^2 s_4 + s_2 (2 s_1 s_3 + s_0 s_4))}{(s_1^2 - s_0 s_2)^2}$$

Deduced from the Liouville-Ostrogradskii formula [compare with the expression(s) above]:

$$\beta_1 = \frac{-s_1^2 + s_0 s_2}{s_0^2}$$

$$\beta_2 = \frac{s_0 (-s_2^3 - s_0 s_3^2 - s_1^2 s_4 + s_2 (2 s_1 s_3 + s_0 s_4))}{(s_1^2 - s_0 s_2)^2}$$

```
In[44]:= Print["The Liouville-Ostrogradskii formula: ", Subscript[P, n - 1], "(z)",
  Subscript[Q, n], "(z) - ", Subscript[P, n], "(z)", Subscript[Q, n - 1],
  "(z) = ", Simplify[LO[n, z], Assumptions -> Subscript[s, 0] > 0]];
n1 = n + 1;
Print["The Liouville-Ostrogradskii formula: ", Subscript[P, n1 - 1], "(z)", Subscript[Q,
  n1], "(z) - ", Subscript[P, n1], "(z)", Subscript[Q, n1 - 1], "(z) = ", LO[n1, z]]
```

The Liouville-Ostrogradskii formula:  $P_1(z)Q_2(z) -$

$$P_2(z)Q_1(z) = \frac{\left(-\frac{s_1^2}{s_0} + s_2\right)^{3/2}}{\sqrt{(s_1^2 - s_0 s_2) (s_2^3 + s_0 s_3^2 + s_1^2 s_4 - s_2 (2 s_1 s_3 + s_0 s_4))}}$$

The Liouville-Ostrogradskii formula:  $P_2(z)Q_3$

$$(z) - P_3(z)Q_2(z) = \left( (s_2^3 + s_0 s_3^2 + s_1^2 s_4 - s_2 (2 s_1 s_3 + s_0 s_4))^2 / \right. \\ \left. (s_0 \sqrt{(s_1^2 - s_0 s_2) (s_2^3 + s_0 s_3^2 + s_1^2 s_4 - s_2 (2 s_1 s_3 + s_0 s_4))} \sqrt{(s_2^3 + s_0 s_3^2 + s_1^2 s_4 - s_2 (2 s_1 s_3 + s_0 s_4))} \right. \\ \left. (-s_4^3 - s_2^2 s_4^2 + s_0 s_4^3 - s_1^2 s_5^2 + s_2^2 s_6 + s_1^2 s_4 s_6 + s_2^2 (3 s_2 s_4 + 2 s_1 s_5 + s_0 s_6) - \right. \\ \left. 2 s_3 ((s_2^2 + s_0 s_4) s_5 + s_1 (s_4^2 + s_2 s_6)) + s_2 (2 s_1 s_4 s_5 + s_0 (s_5^2 - s_4 s_6))) \right) \Bigg)$$

```
In[45]:= Px = Simplify[PnRec[n, z], Assumptions -> {Subscript[s, 0] > 0}];
Qx = Simplify[QnRec[n, z], Assumptions -> {Subscript[s, 0] > 0}];
Qy = Simplify[Qn[n, z, PnRec], Assumptions -> {Subscript[s, 0] > 0}];
Print["(1) Recursively calculated ", Subscript[P, n], "(z) = ", Px];
Print["(2) Directly calculated ", Subscript[P, n], "(z) = ", Pn[n, z]];
Print["(3) Recursively calculated ", Subscript[Q, n], "(z) = ", Qx];
Print["(4) Directly calculated [on the basis of (1)] ",
  Subscript[Q, n], "(z) = ", Qy];
Print["(5) Compare with [directly calculated, on the basis of (2)]: ",
  Subscript[Q, n], "(z) = ", Qn[n, z, Pn]];
Print["One can recursively determine {α1, α2, α3,
  ...} in terms of {s0, s1, s2, ...}, and vice versa."]
```

$$(1) \text{ Recursively calculated } P_2(z) = \frac{z^2 - z \alpha_2 + \alpha_1 (-z + \alpha_2) - \beta_1}{\sqrt{s_0 \beta_1} \sqrt{\beta_2}}$$

$$(2) \text{ Directly calculated } P_2(z) = \frac{-z^2 s_1^2 + z^2 s_0 s_2 + z s_1 s_2 - s_2^2 - z s_0 s_3 + s_1 s_3}{\sqrt{(-s_1^2 + s_0 s_2)} (-s_2^3 + 2 s_1 s_2 s_3 - s_0 s_3^2 - s_1^2 s_4 + s_0 s_2 s_4)}$$

$$(3) \text{ Recursively calculated } Q_2(z) = \frac{z - \alpha_2}{\sqrt{s_0 \beta_1} \sqrt{\beta_2}}$$

$$(4) \text{ Directly calculated [on the basis of (1)] } Q_2(z) = \frac{z - \alpha_2}{\sqrt{s_0 \beta_1} \sqrt{\beta_2}}$$

(5) Compare with [directly calculated, on the basis of (2)]:

$$Q_2(z) = \frac{-s_1^3 + s_0 s_1 (-z s_1 + 2 s_2) + s_0^2 (z s_2 - s_3)}{s_0 \sqrt{(s_1^2 - s_0 s_2)} (s_2^3 + s_0 s_3^2 + s_1^2 s_4 - s_2 (2 s_1 s_3 + s_0 s_4))}$$

One can recursively determine  $\{\alpha_1, \alpha_2, \alpha_3, \dots\}$  in terms of  $\{s_0, s_1, s_2, \dots\}$ , and vice versa.

```
In[46]:= Print["The Liouville-Ostrogradskii formula: ",
  Subscript[P, n - 1], "(z)", Subscript[Q, n], "(z) - ",
  Subscript[P, n], "(z)", Subscript[Q, n - 1], "(z) = ", LOrec[n, z]];
n1 = n + 1;
Print["The Liouville-Ostrogradskii formula: ", Subscript[P, n1 - 1], "(z)", Subscript[Q,
  n1], "(z) - ", Subscript[P, n1], "(z)", Subscript[Q, n1 - 1], "(z) = ", LOrec[n1, z]]
```

$$\text{The Liouville-Ostrogradskii formula: } P_1(z)Q_2(z) - P_2(z)Q_1(z) = \frac{1}{s_0 \sqrt{\beta_2}}$$

$$\text{The Liouville-Ostrogradskii formula: } P_2(z)Q_3(z) - P_3(z)Q_2(z) = \frac{1}{s_0 \sqrt{\beta_3}}$$

```
In[47]:= (* Ref. [125] *)
```

```
In[48]:= Clear[Hmj, Dmj, Aitken, m, j];
Hmj[m_, j_] := Module[(*The (m+1) × (m+1) Hankel moment matrix obtained by
adding j to the indices of the elements of the Hankel
moment matrix Hm. Returns Hm for j=0*) {k, l, T1, T2, hmj}, k = m + 1;
T1 = Table[s1, {l, j, j + k - 1}];
T2 = Table[s1, {l, j + k - 1, j + 2 k - 2}];
hmj = HankelMatrix[T1, T2];
hmj];
Dmj[m_, j_] := Det[Hmj[m, j]];
Aitken[m_, j_] :=
Simplify[Dmj[m, j]^2 - Dmj[m, j - 1] × Dmj[m, j + 1] + Dmj[m + 1, j - 1] × Dmj[m - 1, j + 1]];
```

```
In[49]:= m = 4 (*To be varied*);
j = 2 (*To be varied -- j ≥ 0*);
Print[(Subsuperscript[Δ, m, j])^2, Spacer[1], "-", Spacer[1],
  Subsuperscript[Δ, m, j - 1], Spacer[2], Subsuperscript[Δ, m, j + 1],
  Spacer[1], "+", Spacer[1], Subsuperscript[Δ, m + 1, j - 1],
  Spacer[2], Subsuperscript[Δ, m - 1, j + 1], " = ", Aitken[m, j]]
```

$$(\Delta_4^2)^2 - \Delta_4^1 \Delta_4^3 + \Delta_5^1 \Delta_3^3 = 0$$

```

In[50]:= (* Ref. [127] *)

In[51]:= ClearAll[PrincipalMinors, T1, T2, T3, Hm, m, all];
PrincipalMinors[Hm_, all_] := Module[(*Returns the leading (all) principal
  minors of the (m+1) × (m+1) Hankel matrix Hm for all = 0 (≠ 0).*)
  {mp1, R, n, symb, k, i, j, ss, l, Hx}, mp1 = Length[Hm] (* m+1 *);
  R = Range[mp1];
  If[all == 0, (n = mp1;
    Print[Style["The leading principal minors (PMs):", Gray, Bold, 14]]],
    (n = 2^mp1 - 1;
    Print[Style["All principal minors (PMs):", Gray, Bold, 14]]]);
  symb = If[all == 0, Rotate[Style[α, Bold, 14], 12 Degree],
    Rotate[Style[β, Bold, 14], 12 Degree]];
  k = 0;
  Do[ss = Subsets[R, {i}];
    l = If[all == 0, 1, Length[ss]];
    Do[k = k + 1;
      Hx = Hm[[ss[[j]], ss[[j]]]];
      Print["PM ", k, "/", n, " [", Subscript[symb, k],
        "=", ss[[j]], "]: ", Det[Hx]], {j, 1, l}], {i, 1, mp1}];

In[52]:= m = 2 (*To be varied*);
T1 = Table["G∞"j+1, {j, 1, m}];
T2 = PrependTo[T1, ħ];
T3 = Table["G∞"j+1, {j, m, 2 m}];
Hm = HankelMatrix[T2, T3];
Print["H"m, " = ", MatrixForm[Hm]];

H2 = 
$$\begin{pmatrix} \hbar & G_{\infty 2} & G_{\infty 3} \\ G_{\infty 2} & G_{\infty 3} & G_{\infty 4} \\ G_{\infty 3} & G_{\infty 4} & G_{\infty 5} \end{pmatrix}$$


In[53]:= all = 0 (* = Leading, 1 = All -- To be varied*); PrincipalMinors[Hm, all]

The leading principal minors (PMs):

PM 1/3 [α1 = {1}]: ħ

PM 2/3 [α2 = {1, 2}]: -G∞22 + ħ G∞3

PM 3/3 [α3 = {1, 2, 3}]: -G∞33 + 2 G∞2 G∞3 G∞4 - ħ G∞42 - G∞22 G∞5 + ħ G∞3 G∞5

In[54]:= all = 1 (* = Leading, 1 = All -- To be varied*); PrincipalMinors[Hm, all]

All principal minors (PMs):

PM 1/7 [β1 = {1}]: ħ

PM 2/7 [β2 = {2}]: G∞3

PM 3/7 [β3 = {3}]: G∞5

PM 4/7 [β4 = {1, 2}]: -G∞22 + ħ G∞3

PM 5/7 [β5 = {1, 3}]: -G∞32 + ħ G∞5

PM 6/7 [β6 = {2, 3}]: -G∞42 + G∞3 G∞5

PM 7/7 [β7 = {1, 2, 3}]: -G∞33 + 2 G∞2 G∞3 G∞4 - ħ G∞42 - G∞22 G∞5 + ħ G∞3 G∞5

In[55]:= (* Ref. [128] *)

```

```

In[56]:= ClearAll[rec, Y, NMn, f, r0, r1, n];
rec = Y[k + 1] == (z - Subscript[α, k + 1]) Y[k] - Subscript[β, k] × Y[k - 1];
NMn[n_, {N0_, N1_}] := First[RecurrenceTable[rec && Y[0] == N0 && Y[1] == N1, Y, {k, n, n}]];
f[z_, n_] := Subscript[α, 0] + Subscript[β, 0] × NMn[n, {0, 1}] /
  NMn[n, {1, z - Subscript[α, 1]}] (* alpha_0 + beta_0 N_n(z) / M_n(z) *);

In[57]:= Needs["SymbolicC`"]

In[58]:= n = 3 (*To be varied*);

In[59]:= r0 = f[z, n];
Print[Superscript[ $\tilde{f}$ , CParentheses[n] // ToCodeString], "(z) = ", r0]


$$\tilde{f}^{(3)}(z) = \alpha_0 + \frac{\beta_0 ((z - \alpha_2)(z - \alpha_3) - \beta_2)}{(z - \alpha_3)((z - \alpha_1)(z - \alpha_2) - \beta_1) - (z - \alpha_1)\beta_2}$$


In[60]:= r1 = Apart[r0, z];
Print[Superscript[ $\tilde{f}$ , CParentheses[n] // ToCodeString], "(z) = ", r1]


$$\tilde{f}^{(3)}(z) = \alpha_0 + \frac{z^2 \beta_0 - z \alpha_2 \beta_0 - z \alpha_3 \beta_0 + \alpha_2 \alpha_3 \beta_0 - \beta_0 \beta_2}{z^3 - z^2 \alpha_1 - z^2 \alpha_2 + z \alpha_1 \alpha_2 - z^2 \alpha_3 + z \alpha_1 \alpha_3 + z \alpha_2 \alpha_3 - \alpha_1 \alpha_2 \alpha_3 - z \beta_1 + \alpha_3 \beta_1 - z \beta_2 + \alpha_1 \beta_2}$$


In[61]:= ClearAll[f, r2, s0];
f[z_, n_] := Subscript[α, 0] - ContinuedFractionK[-Subscript[β, j - 1],
  z - Subscript[α, j], {j, 1, n}] (* Continued-fraction expansion *);

In[62]:= s0 = f[z, n] (* Continued-fraction expansion *);
Print[Superscript[ $\tilde{f}$ , CParentheses[n] // ToCodeString], "(z) = ", s0]


$$\tilde{f}^{(3)}(z) = \alpha_0 + \frac{\beta_0}{z - \alpha_1 - \frac{\beta_1}{z - \alpha_2 - \frac{\beta_2}{z - \alpha_3}}}$$


In[63]:= r2 = Apart[s0, z];
Print[Superscript[ $\tilde{f}$ , CParentheses[n] // ToCodeString], "(z) = ", r2]


$$\tilde{f}^{(3)}(z) = \alpha_0 + \frac{z^2 \beta_0 - z \alpha_2 \beta_0 - z \alpha_3 \beta_0 + \alpha_2 \alpha_3 \beta_0 - \beta_0 \beta_2}{z^3 - z^2 \alpha_1 - z^2 \alpha_2 + z \alpha_1 \alpha_2 - z^2 \alpha_3 + z \alpha_1 \alpha_3 + z \alpha_2 \alpha_3 - \alpha_1 \alpha_2 \alpha_3 - z \beta_1 + \alpha_3 \beta_1 - z \beta_2 + \alpha_1 \beta_2}$$


In[64]:= Simplify[r1 - r2] (* Test - Correct outcome: 0 *)

Out[64]= 0

In[65]:= ClearAll[rec, PQn, f, r3, r4];
rec = Sqrt[Subscript[β, k]] y[k - 1] +
  Subscript[α, k + 1] × y[k] + Sqrt[Subscript[β, k + 1]] y[k + 1] == z y[k];
PQn[n_, {PQ0_, PQ1_}] := First[RecurrenceTable[
  rec && y[0] == PQ0 && y[1] == PQ1, y, {k, n, n}]];
f[z_, n_] := Subscript[α, 0] + Subscript[β, 0] × PQn[n,
  {0, 1 / Sqrt[Subscript[s, 0] × Subscript[β, 1]]}] / PQn[n, {1 / Sqrt[Subscript[s, 0]],
  (z - Subscript[α, 1]) / Sqrt[Subscript[s, 0] × Subscript[β, 1]]}]
(* alpha_0 + beta_0 Q_n(z) / P_n(z) -- notice independence on the value of s_0 *);

```

```
In[66]:= r3 = Simplify[f[z, n], Assumptions → {Subscript[s, 0] > 0}];
```

```
Print[Superscript[ $\tilde{f}$ , CParentheses[n] // ToCodeString], "(z) = ", r3]
```

$$\tilde{f}^{(3)}(z) = \alpha_0 + \frac{\beta_0 (z^2 - z \alpha_3 + \alpha_2 (-z + \alpha_3) - \beta_2)}{z^3 - z^2 \alpha_3 + z \alpha_2 (-z + \alpha_3) - z \beta_1 + \alpha_3 \beta_1 - z \beta_2 + \alpha_1 (-z^2 + \alpha_2 (z - \alpha_3) + z \alpha_3 + \beta_2)}$$

```
In[67]:= r4 = Apart[r3, z];
```

```
Print[Superscript[ $\tilde{f}$ , CParentheses[n] // ToCodeString], "(z) = ", r4]
```

$$\tilde{f}^{(3)}(z) = \alpha_0 + \frac{z^2 \beta_0 - z \alpha_2 \beta_0 - z \alpha_3 \beta_0 + \alpha_2 \alpha_3 \beta_0 - \beta_0 \beta_2}{z^3 - z^2 \alpha_1 - z^2 \alpha_2 + z \alpha_1 \alpha_2 - z^2 \alpha_3 + z \alpha_1 \alpha_3 + z \alpha_2 \alpha_3 - \alpha_1 \alpha_2 \alpha_3 - z \beta_1 + \alpha_3 \beta_1 - z \beta_2 + \alpha_1 \beta_2}$$

```
In[68]:= Simplify[r1 - r4] (* Test - Correct outcome: 0 *)
```

```
Out[68]= 0
```

```
In[69]:= (* Ref. [132] *)
```

```
In[70]:= ClearAll[p, q, w];
```

```
p[z_, zeta_, n_] := ChebyshevT[n, z] - zeta ChebyshevT[n - 1, z] (* Pn(z) *);
```

```
q[z_, zeta_, n_] := ChebyshevU[n - 1, z] - zeta ChebyshevU[n - 2, z] (* Qn(z) *);
```

```
w[z_, zeta_, n_] := -q[z, zeta, n] / p[z, zeta, n] (* wn(z) *);
```

```
In[71]:= (* Ref. [133] *)
```

```
In[72]:= ClearAll[rec, f, y, j, Tn, Un, n, T, U];
```

```
rec = y[j - 1] / 2 + y[j + 1] / 2 == z y[j];
```

```
f[n_, {y0_, y1_}] := First[RecurrenceTable[rec && y[0] == y0 && y[1] == y1, y, {j, n, n}]];
```

```
Tn[n_, z_] := Expand[f[n, {1, z}], z];
```

```
Un[n_, z_] := Expand[f[n, {1, 2 z}], z];
```

```
In[73]:= (* Illustration *)
```

```
In[74]:= n = 10 (* To be varied *);
```

```
In[75]:= Print[Subscript[T, n], "(z) = ", Tn[n, z], " (Recursively determined)";
```

```
Print[Subscript[T, n], "(z) = ", ChebyshevT[n, z], " (Standard)";
```

```
Print[Subscript[U, n], "(z) = ", Un[n, z], " (Recursively determined)";
```

```
Print[Subscript[U, n], "(z) = ", ChebyshevU[n, z], " (Standard)";
```

$$T_{10}(z) = -1 + 50 z^2 - 400 z^4 + 1120 z^6 - 1280 z^8 + 512 z^{10} \quad (\text{Recursively determined})$$

$$T_{10}(z) = -1 + 50 z^2 - 400 z^4 + 1120 z^6 - 1280 z^8 + 512 z^{10} \quad (\text{Standard})$$

$$U_{10}(z) = -1 + 60 z^2 - 560 z^4 + 1792 z^6 - 2304 z^8 + 1024 z^{10} \quad (\text{Recursively determined})$$

$$U_{10}(z) = -1 + 60 z^2 - 560 z^4 + 1792 z^6 - 2304 z^8 + 1024 z^{10} \quad (\text{Standard})$$

```
In[76]:= (* Ref. [134] *)
```

```

In[77]:= ClearAll[p, q, w, sj, n, j, j1, t];
p[z_, t_, n_] := ChebyshevT[n, z] - t ChebyshevT[n - 1, z] (*Pn(z)*);
q[z_, t_, n_] := ChebyshevU[n - 1, z] - t ChebyshevU[n - 2, z] (*Qn(z)*);
w[z_, t_, n_] := -q[z, t, n] / p[z, t, n] (*wn(z, τ)*);
sj[j_, t_, n_] := Module[{f, sol, z, x, k},
  sol = z /. NSolve[p[z, t, n + 1] == 0 && -1 ≤ z ≤ 1, z, WorkingPrecision → 120];
  Do[x[k] = Residue[-w[z, t, n + 1], {z, sol[[k]]}], {k, 1, n + 1}];
  f = Sum[x[k] * sol[[k]]^j, {k, 1, n + 1}] (*Eq. (B.107)*);
  f] (*Returns the coefficient of 1/zj+1 in the asymptotic series expansion of -
  wn+1(z, τ) for z → ∞.*);

In[81]:= n = 4 (*To be varied*);

In[82]:= Print[Subscript[-w̃, n + 1], "(z, τ) ~ ",
  Simplify[Series[-w[z, τ, n + 1], {z, Infinity, 2 n + 4}]], " for z → ∞."]

$$-\tilde{w}_5(z, \tau) \sim \frac{1}{z} + \frac{1}{2z^3} + \frac{3}{8z^5} + \frac{5}{16z^7} + \frac{35}{128z^9} + \frac{\tau}{256z^{10}} + \frac{125 + \tau^2}{512z^{11}} + \frac{\tau(10 + \tau^2)}{1024z^{12}} + O\left[\frac{1}{z}\right]^{13} \text{ for } z \rightarrow \infty.$$


In[83]:= (* Test *)

In[84]:= t = 1 (*Do not change*);
j = 6 (*To be varied*);
j1 = j + 1;
Print[Subscript[c, j1], " = ", Rationalize[sj[j, t, n]]]
(*The coefficient of 1/z{j+1}*)

$$c_7 = \frac{5}{16}$$


In[85]:= Print["Explicitly-calculated value for ", Subscript[c, j1], " = ",
  (1 - (-1)^j1) Gamma[j1 / 2] / (2 Sqrt[Pi] Gamma[(j1 + 1) / 2])] (*Eq. (B.169)*)
Explicitly-calculated value for c7 =  $\frac{5}{16}$ 

In[86]:= (* §§ 3.3.1 and B.4 of the
  publication: - Not included in the body of the publication *)

```

```

In[87]:= ClearAll[P, Q, p, q, w, wct, rc];
P[z_, n_] := ChebyshevT[n, z] (*  $P_n(z)$  *);
Q[z_, n_] := ChebyshevU[n - 1, z] (*  $Q_n(z)$  *);
p[z_, tau_, n_] := P[z, n] - tau P[z, n - 1] (*  $P_n(z, \tau)$  *);
q[z_, tau_, n_] := Q[z, n] - tau Q[z, n - 1] (*  $Q_n(z, \tau)$  *);
w[z_, tau_, n_] := -q[z, tau, n] / p[z, tau, n] (*  $w_n(z, \tau)$  *);
wct[z_, n_] := -(Q[z, n] Conjugate[P[z, n - 1]] - Q[z, n - 1] Conjugate[P[z, n]]) / (P[z, n]
  Conjugate[P[z, n - 1]] - P[z, n - 1] Conjugate[P[z, n]]) (*The centre  $w_n^c(z)$  of the
  circle traversed by  $w_n(z, \tau)$  on increasing  $\tau$  from  $-\infty$  to  $+\infty$  - Independent of  $\tau$  *);
rc[z_, n_] := 1 / (Abs[z - Conjugate[z]] (1 + 2 Sum[Abs[P[z, j]]^2, {j, 1, n - 1}]))
(*The radius of the circle [Eq. (B.177)] traversed by  $w_n(z, \tau)$  on increasing  $\tau$  from  $-\infty$  to  $+\infty$  using the Christoffel-Darboux formula appropriate for the case at hand,
where  $T_0(x)$  is normalised differently than  $T_j(x)$ ,  $j = 1, 2, 3, \dots$ . The validity
of this expression can be tested with the aid of the function rcx[z,n]*);
rcx[z_, n_] := Abs[(Q[z, n]  $\times$  P[z, n - 1] - Q[z, n - 1]  $\times$  P[z, n]) /
  (P[z, n] Conjugate[P[z, n - 1]] - P[z, n - 1] Conjugate[P[z, n]])]
(*The radius of the circle [Eq. (B.174)] traversed by  $w_n(z, \tau)$  on increasing  $\tau$  from  $-\infty$  to  $+\infty$  without using the Christoffel-Darboux formula*);

```

In[88]:= (\*Below,

the arrows on each circular contour show the direction of progression of the mapping  $-w_n(z, \tau)$  for  $\tau$  increasing from the given lowest to the given highest value. For  $\text{Im}[z] > 0$  ( $\text{Im}[z] < 0$ ) this direction, or orientation, must be clockwise (anticlockwise). To appreciate this, see the discussions regarding the Möbius transformation  $w_{n+1}(z, \xi)$  in § 3.3.1 of the publication, beginning from Eq. (3.18). Briefly, with the  $\tau$ -axis representing the real axis of the  $\xi$ -plane, for  $\tau$  increasing from  $-\infty$  to  $+\infty$  the upper (lower) half of the  $\xi$ -plane becomes the interior of a circle of infinite radius traversed anticlockwise (clockwise). Let us consider the upper half of the  $\xi$ -plane as the interior of the just-mentioned circle, whereby the direction of  $\tau$  increasing from  $-\infty$  to  $+\infty$  amounts to an anticlockwise circulation (the conclusion is independent of this choice). Since  $v_n(z)$  (the simple pole of the relevant Möbius transformation in the  $\xi$ -plane) is a Nevanlinna function of  $z$ ,  $v_n(z)$  is in the same half-plane as  $z$ . Thus, for  $\text{Im}[z] > 0$  ( $\text{Im}[z] < 0$ ),  $v_n(z)$  is in the interior (exterior) region of the above-mentioned circle of infinite radius. It follows that for  $\text{Im}[z] > 0$  ( $\text{Im}[z] < 0$ ) the orientation of the circular trajectory of the mapping  $-w_n(z, \tau)$  (and similarly  $w_n(z, \tau)$  -- note that multiplication by  $-1$  amounts to a reflection in the origin of the  $w$ -plane, so that it does not change orientation, nor does it effect change of interior into exterior, and vice versa) is opposite (the same as) that of  $\tau$  along the real  $\tau$ -axis, which we have assumed to be anticlockwise. Note that for  $\text{Im}[z] > 0$  ( $\text{Im}[z] < 0$ ) the mapping  $-w_n(z, \xi)$  (as well as  $w_n(z, \xi)$ ) maps the lower (upper) half of the  $\xi$ -plane into the interior of the oriented circle in the  $w$ -plane displayed below. This is important for the (uniform) convergence of  $-w_{n+1}(z, \tau)$  to  $-w(z)$  for  $n \rightarrow \infty$ . This follows from the fact that the remainder of the approximant  $-w_n(z, \tau)$  is, similarly to  $-w(z)$ , located in the lower (upper) half-plane for  $\text{Im}[z] > 0$  ( $\text{Im}[z] < 0$ ). \*)

In[89]:= (\* The following two examples show the convergence behaviour of  $-$

$w_n(z, \tau)$  (towards  $-w(z)$ ) for three consecutive values of  $n$ :  $n$ ,  $n+1$ , and  $n+2$ . In the first example  $z$  is just above the branch cut of  $w(z)$  (which covers the interval  $[-1, +1]$ ) and in the second example, away from it (See the discussions centred on Eq. (B.112) and §§ B.1.1 and B.4 of the publication). We point out that since  $w(z)$  is a Nevanlinna function of  $z$ , we consider  $-w(z)$  in order to make contact with the Green function  $G(z)$  and the self-energy  $\Sigma(z)$  whose negatives are Nevanlinna functions of  $z$ . Note that the circle corresponding to  $n+1$  is interior to that corresponding to  $n$ , and the two circles touch at one point. Similarly as regards the circles corresponding to  $n+1$  and  $n+2$ . \*)

```

In[90]:= ClearAll[n, z, taumin, taumax, mwz];
n = 20 (*To be varied*);
z = (0.5 + 0.05 I) (*To be varied*);
taumin = -100 (*Minimum value of  $\tau$  - To be varied*);
taumax = 100 (*Maximum value of  $\tau$  - To be varied*);
mwz = 1 / (z Sqrt[1 - 1 / z^2]) (* -w(z) *);
Print["n: ", Style[n, Red], ", z: ", Style[z, Red]];
Print["The origin of the coordinate system (value of the exact -w(z) = -w∞(z)): ",
Style[mwz, Red]];
Print["The centre of the inner circle, -wn+2c(z): ", Style[-wct[z, n + 2], Red]];
Print["The Radius of the inner circle,  $\rho_{n+2}^c(z)$ : ", Style[rcx[z, n + 2], Red]];
Show[ParametricPlot[{{(*1*)Re[-w[z, tau, n]], Im[-w[z, tau, n]]},
{(*2*)Re[-w[z, tau, n + 1]], Im[-w[z, tau, n + 1]]}, {(*3*)Re[-w[z, tau, n + 2]],
Im[-w[z, tau, n + 2]]}}, {tau, taumin, taumax}, PlotStyle → {Directive[(*1*)
Darker[Green], Thin], Directive[(*2*)Blue, Thin], Directive[(*3*)Red,
Thin]}, PlotRange → All, MaxRecursion → 15, AxesOrigin → {Re[mwz], Im[mwz]},
AxesLabel → {Re, Im}, PlotLabel → "w-plane", PlotLegends → {Style["-wn(z,  $\tau$ )", Darker[
Green], 12], Style["-wn+1(z,  $\tau$ )", Blue, 12], Style["-wn+2(z,  $\tau$ )", Red, 12]}] /.
Line[x_] → {Arrowheads[{0.02, 0.02, 0.02, 0.02}], Arrow[x]}

```

n: 20, z: 0.5 + 0.05 i

The origin of the coordinate system (value of the exact -w(z) = -w<sub>∞</sub>(z)):

0.0381931 - 1.15088 i

The centre of the inner circle, -w<sub>n+2</sub><sup>c</sup>(z): 0.0324126 - 1.15584 i

The Radius of the inner circle,  $\rho_{n+2}^c(z)$ : 0.192764

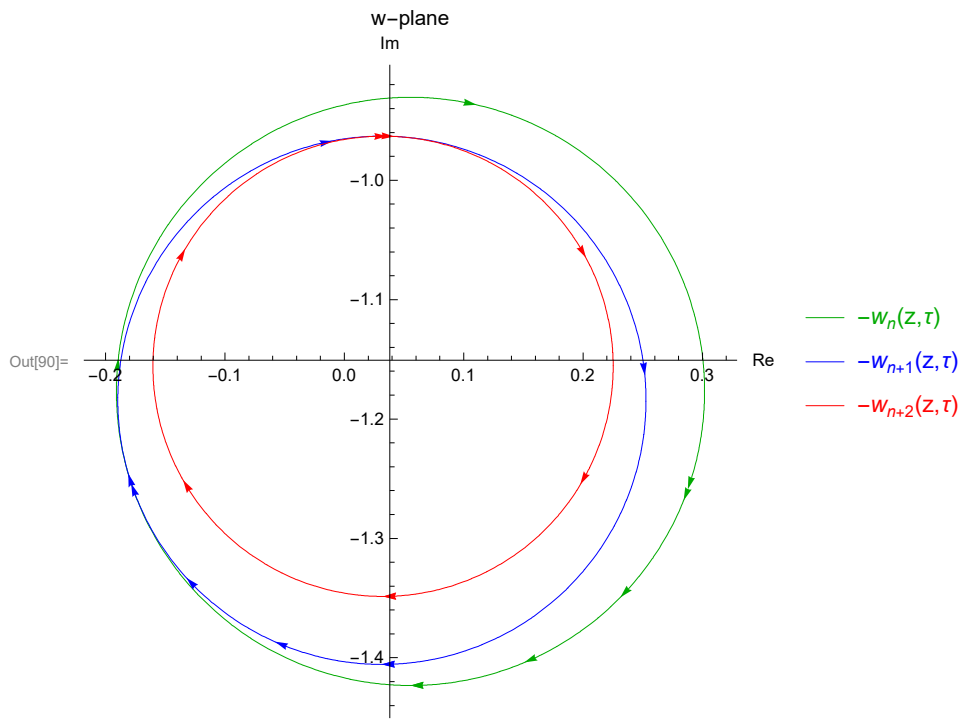

In[91]:= (\* Test \*)

```

In[92]:= Print["Radius of the inner circle. Direct expression: ", Style[rcx[z, n + 2], Red],
  ". Using the Christoffel-Darboux formula: ", Style[rc[z, n + 2], Red]]

Radius of the inner circle. Direct expression:
0.192764. Using the Christoffel-Darboux formula: 0.192764

In[93]:= (* End test *)

In[94]:= ClearAll[n, z, taumin, taumax, mwz];
n = 5 (*To be varied*);
z = (1.5 + 0.05 I) (*To be varied*);
taumin = -100 (*Minimum value of  $\tau$  - To be varied*);
taumax = 100 (*Maximum value of  $\tau$  - To be varied*);
mwz = 1 / (z Sqrt[1 - 1 / z^2]) (* -w(z) *);
Print["n: ", Style[n, Red], ", z: ", Style[z, Red]];
Print["The origin of the coordinate system (value of the exact  $-w(z) = -w_\infty(z)$ ): ",
  Style[mwz, Red]];
Print["The centre of the inner circle,  $-w_{n+2}^c(z)$ : ", Style[-wct[z, n + 2], Red]];
Print["The Radius of the inner circle,  $\rho_{n+2}^c(z)$ : ", Style[rc[z, n + 2], Red]];
Show[ParametricPlot[{{(*1*)Re[-w[z, tau, n]], Im[-w[z, tau, n]]},
  {(*2*)Re[-w[z, tau, n + 1]], Im[-w[z, tau, n + 1]]}, {(*3*)Re[-w[z, tau, n + 2]],
  Im[-w[z, tau, n + 2]]}}, {tau, taumin, taumax}, PlotStyle -> {Directive[(*1*)
  Darker[Green], Thin], Directive[(*2*)Blue, Thin], Directive[(*3*)Red,
  Thin]}, PlotRange -> All, MaxRecursion -> 15, AxesOrigin -> {Re[mwz], Im[mwz]},
  AxesLabel -> {Re, Im}, PlotLabel -> "w-plane", PlotLegends -> {Style["-w_n(z,  $\tau$ )", Darker[
  Green], 12], Style["-w_{n+1}(z,  $\tau$ )", Blue, 12], Style["-w_{n+2}(z,  $\tau$ )", Red, 12]}] /.
  Line[x_] -> {Arrowheads[{0.02, 0.02, 0.02, 0.02}], Arrow[x]}]

```

n: 5, z: 1.5 + 0.05 i

The origin of the coordinate system (value of the exact  $-w(z) = -w_\infty(z)$ ):

0.890519 - 0.0533461 i

The centre of the inner circle,  $-w_{n+2}^c(z)$ : 0.890423 - 0.0534761 i

The Radius of the inner circle,  $\rho_{n+2}^c(z)$ : 0.000162189

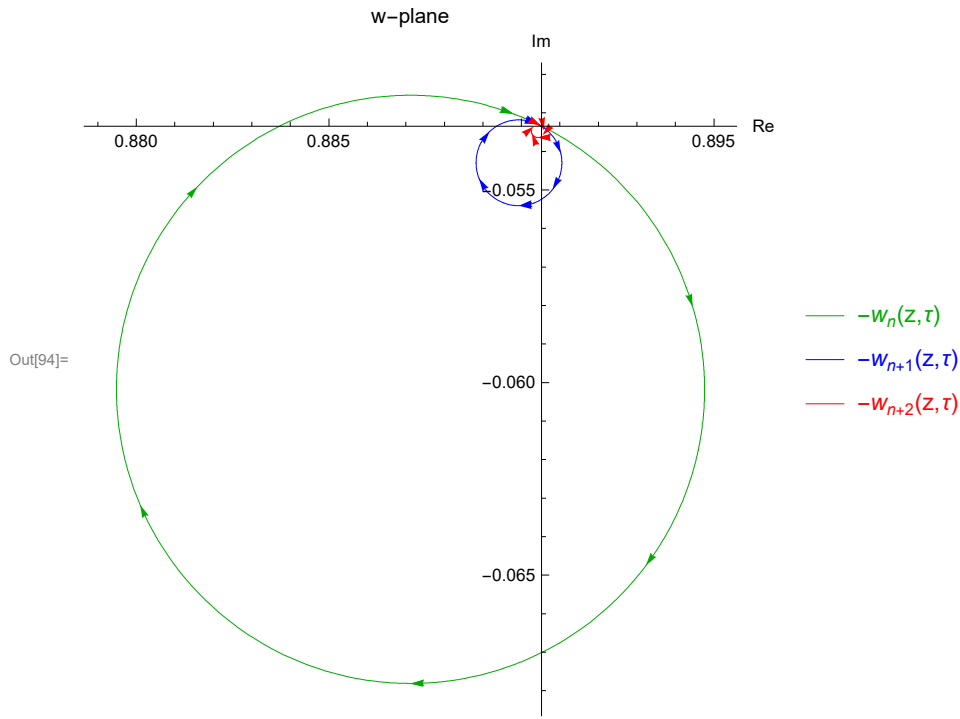

In[95]:= (\* Test \*)

In[96]:= Print["Radius of the inner circle. Direct expression: ", Style[rcx[z, n + 2], Red],  
". Using the Christoffel-Darboux formula: ", Style[rc[z, n + 2], Red]]

Radius of the inner circle. Direct expression:

0.000162189. Using the Christoffel-Darboux formula: 0.000162189

In[97]:= (\* End test \*)

In[98]:= (\* Symbolic computation -  
Programs Equiv and Verify included in § D.4 of appendix D \*)

In[99]:= ClearAll[Verify, Equiv];  
Verify[xia\_, sig\_] :=  
Module[{len, nu, xo, y, y1, xo1, xo2, x, x1, x2, ze, i, p0, fx, fp}, len = Length[xia];  
nu = (len + 1) / 2;  
xo = Table[0, {i, 1, len}];  
fx := Function[{i}, ToExpression["x" <> ToString[#]] & /@ Range[i]];  
fp := Function[{i}, ToExpression["p" <> ToString[#]] & /@ Range[i]];  
x = fx[nu];  
y = fp[nu];  
y1 = Table[y[[i]] -> y[[i]] + x[[i]] "p0", {i, 1, nu}];  
Do[If[sig[[i]] == -1, xo[[i]] = xia[[i]] + "p0", xo[[i]] = xia[[i]]], {i, 1, len}];  
xo1 = xo /. y1;  
xo2 = Simplify[(xo1 - xia) / "p0"];

```

ze = Table[0, {i, 1, len}];
x1 = Solve[xo2 == ze, x, Integers];
x2 = Table[x1[[1, i, 2]], {i, 1, nu}]; x2];
Equiv[ML_, MS_, nu_, p_, xi_, phs_, all_] :=
Module[{i, j, k, l, m, n, n1, nf, q, v, xo, y, s, sig, g, h, T, T0, T1,
  T2, S0, SIG, ONE, Vr}, Print[Style["Program Equiv", Gray, Bold, 16]];
Print[Style[DateString[], Gray]];
Print["v: ", nu, ". Particle-hole symmetry? ",
  If[phs == 0, Style[No, Red], Style[Yes, Red]], " | Search for all possibilities? ",
  If[all == 0, Style[No, Red], Style[Yes, Red]]];
n =
  2
  nu - 1;
n1 = n;
nf = n!;
v = Join[{p, p}, Table[0, {i, 1, n - 1}]];
ONE = Table[1, {i, 1, n}];
Do[h[i] = i, {i, 1, n}]; If[phs == 0, 99, (S0 = DeleteDuplicates[xi];
  n1 = Count[S0, Except[-1000]];
  If[n1 == n, 98,
    (Do[Do[If[SameQ[xi[[i]], S0[[k]]], (h[i] = k), 97], {k, 1, n1}], {i, 1, n})]]];
T0 = Range[n]; If[phs == 0, (m = 1), (m = 2^n1)];
Print["Number of Green functions  $\nu' = 2\nu - 1$  ( $2^{\nu'}$ ): ",
  Style[n1, Red], " (" , 2^n1, ")"];
q = 0;
Do[If[nu > 3, (PrintTemporary["→ 1 = ", 1, "/", m]), 96];
  s = IntegerDigits[1 - 1, 2, n1];
  Do[T = Table[(-1)^s[[h[i]]] xi[[i]], {i, 1, n}];
    T1 = Table[T[[Permutations[T0][[j, i]]]], {i, 1, n}];
    T2 = Simplify[MS.T1]; xo = Join[T1, T2]; y = ML.xo; g = True;
    Do[g = g && SameQ[Simplify[v[[i]] - y[[i]], 0], {i, 1, n}];
    If[g, (q = q + 1;
      sig = 1;
      Do[sig = sig * (-1)^(s[[h[i]]]), {i, 1, n}];
      SIG = Table[(-1)^s[[h[i]]], {i, 1, n}];
      Print[" $\Rightarrow$  1, j = ", 1, ", ", j,
        ".  $\vec{S} = (s_1, s_2, \dots, s_{2\nu-1})$ : ", SIG, ".  $s$ : ", Style[sig, Red], ".");
      If[SIG != ONE, (Vr = Verify[xi, SIG];
        Print[Style["Verification  $\Rightarrow$ ", Darker[Green], Plain, 12],
          " { $\alpha_1, \alpha_2, \dots, \alpha_\nu$ }: ", Vr]), 100];
      Do[Print[Subscript[x, i], ": ", Style[xo[[i]], Blue]], {i, 1, n}];
      Do[Print[Subscript[x, i], ": ", xo[[i]], {i, n + 1, n + nu}];
      If[all == 0, Goto[end], 95]), 94], {j, 1, nf}], {1, 1, m}];
Label[end];
Print["Number of distinct outputs: ",
  Style[q, Red], ". (If 0, diagrams A and B are not equivalent.)"];
Print[Style[DateString[], Gray]];
xo;];

```

```

In[101]:= (* Illustrative examples *)

In[102]:= (* Example 1 - Concerns  $\Sigma^{2.1}(2',1')$ , as diagram A,
and  $\Sigma^{2.2}(2',1')$ , as daigram B | Fig. 15 *)

In[103]:= Clear[p, p1, p2, xi, ML, MS];
nu = 2 (*Order of the diagrams*);
phs = 1(*0=No p-h symmetry; 1=p-h symmetry*); all = 1
(*0, Do not search for all; 1, Search for all*);
xi = {p1, p2, p - p1 + p2}; Print[" $\vec{\xi} =$ ", MatrixForm[xi]];
ML = SparseArray[{{1, 1} → 1, {1, 4} → 1, {2, 1} → 1, {2, 5} → 1,
{3, 2} → 1, {3, 3} → -1, {3, 5} → 1, {4, 2} → 1, {4, 3} → -1, {4, 4} → 1}];
Print[" $M_L =$ ", MatrixForm[ML]];
MS = SparseArray[{{1, 2} → -1, {1, 3} → 1, {2, 2} → -1, {2, 3} → 1}];
Print[" $M_S =$ ", MatrixForm[MS]];
Equiv[ML, MS, nu, p, xi, phs, all]

```

$$\vec{\xi} = \begin{pmatrix} p_1 \\ p_2 \\ p - p_1 + p_2 \end{pmatrix}$$

$$M_L = \begin{pmatrix} 1 & 0 & 0 & 1 & 0 \\ 1 & 0 & 0 & 0 & 1 \\ 0 & 1 & -1 & 0 & 1 \\ 0 & 1 & -1 & 1 & 0 \end{pmatrix}$$

$$M_S = \begin{pmatrix} 0 & -1 & 1 \\ 0 & -1 & 1 \end{pmatrix}$$

### Program Equiv

Tue 24 Aug 2021 11:39:33

$v$ : 2. Particle-hole symmetry? **Yes** | Search for all possibilities? **Yes**

Number of Green functions  $v' = 2v - 1$  ( $2^{v'}$ ): **3** (8)

$\Rightarrow 1, j = 1, 1. \vec{\zeta} = (\zeta_1, \zeta_2, \dots, \zeta_{2v-1}): \{1, 1, 1\}. \zeta: \mathbf{1}.$

$x_1$ :  $p_1$

$x_2$ :  $p_2$

$x_3$ :  $p - p_1 + p_2$

$x_4$ :  $p - p_1$

$x_5$ :  $p - p_1$

$\Rightarrow 1, j = 1, 6. \vec{\zeta} = (\zeta_1, \zeta_2, \dots, \zeta_{2v-1}): \{1, 1, 1\}. \zeta: \mathbf{1}.$

$x_1$ :  $p - p_1 + p_2$

$x_2$ :  $p_2$

$x_3$ :  $p_1$

$x_4$ :  $p_1 - p_2$

$x_5$ :  $p_1 - p_2$

$\Rightarrow 1, j = 4, 2. \vec{\zeta} = (\zeta_1, \zeta_2, \dots, \zeta_{2v-1}): \{1, -1, -1\}. \zeta: \mathbf{1}.$

Verification  $\Rightarrow \{\alpha_1, \alpha_2, \dots, \alpha_v\}: \{0, -1\}$

$x_1$ :  $p_1$

$$x_2: -p + p1 - p2$$

$$x_3: -p2$$

$$x_4: p - p1$$

$$x_5: p - p1$$

$$\Rightarrow 1, j = 4, 4. \vec{\zeta} = (\zeta_1, \zeta_2, \dots, \zeta_{2v-1}): \{1, -1, -1\}. \zeta: 1.$$

$$\text{Verification} \Rightarrow \{\alpha_1, \alpha_2, \dots, \alpha_v\}: \{0, -1\}$$

$$x_1: -p2$$

$$x_2: -p + p1 - p2$$

$$x_3: p1$$

$$x_4: p + p2$$

$$x_5: p + p2$$

$$\Rightarrow 1, j = 7, 3. \vec{\zeta} = (\zeta_1, \zeta_2, \dots, \zeta_{2v-1}): \{-1, -1, 1\}. \zeta: 1.$$

$$\text{Verification} \Rightarrow \{\alpha_1, \alpha_2, \dots, \alpha_v\}: \{-1, -1\}$$

$$x_1: -p2$$

$$x_2: -p1$$

$$x_3: p - p1 + p2$$

$$x_4: p + p2$$

$$x_5: p + p2$$

$$\Rightarrow 1, j = 7, 5. \vec{\zeta} = (\zeta_1, \zeta_2, \dots, \zeta_{2v-1}): \{-1, -1, 1\}. \zeta: 1.$$

$$\text{Verification} \Rightarrow \{\alpha_1, \alpha_2, \dots, \alpha_v\}: \{-1, -1\}$$

$$x_1: p - p1 + p2$$

$$x_2: -p1$$

$$x_3: -p2$$

$$x_4: p1 - p2$$

$$x_5: p1 - p2$$

Number of distinct outputs: 6. (If 0, diagrams A and B are not equivalent.)

Tue 24 Aug 2021 11:39:33

In[107]:= (\* **Example 2** - Concerns  $\Sigma^{\{4.40\}}(2', 1')$ , as diagram A,  
and  $\Sigma^{\{4.79\}}(2', 1')$ , as daigram B | **Fig. 16** \*)

```

In[108]:= Clear[p, p1, p2, p3, p4, xi, ML, MS];
nu = 4 (*Order of the diagrams*);
phs = 1 (*0=No p-h symmetry; 1 = p-h symmetry*);
all = 1 (*0, Do not search for all; 1, Search for all*);
xi = {p1, p2, p3, p4, p1 - p2 + p4, p - p2 + p4, p - p3 + p4};
Print[" $\vec{\xi} =$ ", MatrixForm[xi]];
ML = SparseArray[{{1, 1} → 1, {1, 8} → 1, {2, 3} → 1, {2, 11} → 1,
  {3, 1} → 1, {3, 2} → -1, {3, 9} → -1, {4, 2} → 1, {4, 3} → -1, {4, 10} → 1,
  {5, 4} → 1, {5, 5} → -1, {5, 11} → 1, {6, 4} → 1, {6, 5} → -1, {6, 9} → 1,
  {7, 6} → 1, {7, 7} → -1, {7, 10} → 1, {8, 6} → 1, {8, 7} → -1, {8, 8} → 1}];
Print[" $M_L =$ ", MatrixForm[ML]];
MS = SparseArray[{{1, 6} → -1, {1, 7} → 1, {2, 4} → -1,
  {2, 5} → 1, {3, 6} → -1, {3, 7} → 1, {4, 4} → -1, {4, 5} → 1}];
Print[" $M_S =$ ", MatrixForm[MS]];
Equiv[ML, MS, nu, p, xi, phs, all]

```

$$\vec{\xi} = \begin{pmatrix} p1 \\ p2 \\ p3 \\ p4 \\ p1 - p2 + p4 \\ p - p2 + p4 \\ p - p3 + p4 \end{pmatrix}$$

$$M_L = \begin{pmatrix} 1 & 0 & 0 & 0 & 0 & 0 & 0 & 1 & 0 & 0 & 0 \\ 0 & 0 & 1 & 0 & 0 & 0 & 0 & 0 & 0 & 0 & 1 \\ 1 & -1 & 0 & 0 & 0 & 0 & 0 & 0 & -1 & 0 & 0 \\ 0 & 1 & -1 & 0 & 0 & 0 & 0 & 0 & 0 & 1 & 0 \\ 0 & 0 & 0 & 1 & -1 & 0 & 0 & 0 & 0 & 0 & 1 \\ 0 & 0 & 0 & 1 & -1 & 0 & 0 & 0 & 1 & 0 & 0 \\ 0 & 0 & 0 & 0 & 0 & 1 & -1 & 0 & 0 & 1 & 0 \\ 0 & 0 & 0 & 0 & 0 & 1 & -1 & 1 & 0 & 0 & 0 \end{pmatrix}$$

$$M_S = \begin{pmatrix} 0 & 0 & 0 & 0 & 0 & -1 & 1 \\ 0 & 0 & 0 & -1 & 1 & 0 & 0 \\ 0 & 0 & 0 & 0 & 0 & -1 & 1 \\ 0 & 0 & 0 & -1 & 1 & 0 & 0 \end{pmatrix}$$

## Program Equiv

Tue 24 Aug 2021 11:39:33

v: 4. Particle-hole symmetry? **Yes** | Search for all possibilities? **Yes**

Number of Green functions  $v' = 2v - 1$  ( $2^{v'}$ ): **7** (128)

$\Rightarrow 1, j = 42, 2366. \vec{\zeta} = (\zeta_1, \zeta_2, \dots, \zeta_{2v-1}): \{1, -1, 1, -1, 1, 1, -1\}. \zeta: -1.$

**Verification**  $\Rightarrow \{\alpha_1, \alpha_2, \dots, \alpha_v\}: \{0, -1, 0, -1\}$

$x_1$ : -p4

$x_2$ : -p2

$x_3$ : p - p2 + p4

$x_4$ : p1 - p2 + p4

$x_5$ : p1

$x_6$ : -p + p3 - p4

$x_7$ : p3

$$x_8: p + p^4$$

$$x_9: p^2 - p^4$$

$$x_{10}: p + p^4$$

$$x_{11}: p^2 - p^4$$

$$\Rightarrow 1, j = 42, 3790. \vec{\zeta} = (\zeta_1, \zeta_2, \dots, \zeta_{2^j-1}): \{1, -1, 1, -1, 1, 1, -1\}. \zeta: -1.$$

$$\text{Verification} \Rightarrow \{\alpha_1, \alpha_2, \dots, \alpha_v\}: \{0, -1, 0, -1\}$$

$$x_1: p - p^2 + p^4$$

$$x_2: -p^2$$

$$x_3: -p^4$$

$$x_4: -p + p^3 - p^4$$

$$x_5: p^3$$

$$x_6: p^1 - p^2 + p^4$$

$$x_7: p^1$$

$$x_8: p^2 - p^4$$

$$x_9: p + p^4$$

$$x_{10}: p^2 - p^4$$

$$x_{11}: p + p^4$$

$$\Rightarrow 1, j = 57, 2365. \vec{\zeta} = (\zeta_1, \zeta_2, \dots, \zeta_{2^j-1}): \{1, -1, -1, -1, 1, 1, 1\}. \zeta: -1.$$

$$\text{Verification} \Rightarrow \{\alpha_1, \alpha_2, \dots, \alpha_v\}: \{0, -1, -1, -1\}$$

$$x_1: -p^4$$

$$x_2: -p^2$$

$$x_3: p - p^2 + p^4$$

$$x_4: p^1 - p^2 + p^4$$

$$x_5: p^1$$

$$x_6: -p^3$$

$$x_7: p - p^3 + p^4$$

$$x_8: p + p^4$$

$$x_9: p^2 - p^4$$

$$x_{10}: p + p^4$$

$$x_{11}: p^2 - p^4$$

$$\Rightarrow 1, j = 57, 3780. \vec{\zeta} = (\zeta_1, \zeta_2, \dots, \zeta_{2^j-1}): \{1, -1, -1, -1, 1, 1, 1\}. \zeta: -1.$$

$$\text{Verification} \Rightarrow \{\alpha_1, \alpha_2, \dots, \alpha_v\}: \{0, -1, -1, -1\}$$

$$x_1: p - p^2 + p^4$$

$$x_2: -p^2$$

$$x_3: -p^4$$

$$x_4: -p^3$$

$$x_5: p - p^3 + p^4$$

$$x_6: p^1 - p^2 + p^4$$

$$x_7: p^1$$

$$x_8: p_2 - p_4$$

$$x_9: p + p_4$$

$$x_{10}: p_2 - p_4$$

$$x_{11}: p + p_4$$

$$\Rightarrow 1, j = 110, 2356. \vec{\zeta} = (\zeta_1, \zeta_2, \dots, \zeta_{2\nu-1}): \{-1, -1, 1, -1, -1, 1, -1\}. \zeta: -1.$$

$$\text{Verification} \Rightarrow \{\alpha_1, \alpha_2, \dots, \alpha_\nu\}: \{-1, -1, 0, -1\}$$

$$x_1: -p_4$$

$$x_2: -p_2$$

$$x_3: p - p_2 + p_4$$

$$x_4: -p_1$$

$$x_5: -p_1 + p_2 - p_4$$

$$x_6: -p + p_3 - p_4$$

$$x_7: p_3$$

$$x_8: p + p_4$$

$$x_9: p_2 - p_4$$

$$x_{10}: p + p_4$$

$$x_{11}: p_2 - p_4$$

$$\Rightarrow 1, j = 110, 3789. \vec{\zeta} = (\zeta_1, \zeta_2, \dots, \zeta_{2\nu-1}): \{-1, -1, 1, -1, -1, 1, -1\}. \zeta: -1.$$

$$\text{Verification} \Rightarrow \{\alpha_1, \alpha_2, \dots, \alpha_\nu\}: \{-1, -1, 0, -1\}$$

$$x_1: p - p_2 + p_4$$

$$x_2: -p_2$$

$$x_3: -p_4$$

$$x_4: -p + p_3 - p_4$$

$$x_5: p_3$$

$$x_6: -p_1$$

$$x_7: -p_1 + p_2 - p_4$$

$$x_8: p_2 - p_4$$

$$x_9: p + p_4$$

$$x_{10}: p_2 - p_4$$

$$x_{11}: p + p_4$$

$$\Rightarrow 1, j = 125, 2355. \vec{\zeta} = (\zeta_1, \zeta_2, \dots, \zeta_{2\nu-1}): \{-1, -1, -1, -1, -1, 1, 1\}. \zeta: -1.$$

$$\text{Verification} \Rightarrow \{\alpha_1, \alpha_2, \dots, \alpha_\nu\}: \{-1, -1, -1, -1\}$$

$$x_1: -p_4$$

$$x_2: -p_2$$

$$x_3: p - p_2 + p_4$$

$$x_4: -p_1$$

$$x_5: -p_1 + p_2 - p_4$$

$$x_6: -p_3$$

$$x_7: p - p_3 + p_4$$

$x_8: p + p^4$

$x_9: p^2 - p^4$

$x_{10}: p + p^4$

$x_{11}: p^2 - p^4$

$\Rightarrow 1, j = 125, 3779. \vec{\zeta} = (\zeta_1, \zeta_2, \dots, \zeta_{2v-1}): \{-1, -1, -1, -1, -1, 1, 1\}. \zeta: -1.$

Verification  $\Rightarrow \{\alpha_1, \alpha_2, \dots, \alpha_v\}: \{-1, -1, -1, -1\}$

$x_1: p - p^2 + p^4$

$x_2: -p^2$

$x_3: -p^4$

$x_4: -p^3$

$x_5: p - p^3 + p^4$

$x_6: -p^1$

$x_7: -p^1 + p^2 - p^4$

$x_8: p^2 - p^4$

$x_9: p + p^4$

$x_{10}: p^2 - p^4$

$x_{11}: p + p^4$

Number of distinct outputs: 8. (If 0, diagrams A and B are not equivalent.)

Tue 24 Aug 2021 11:42:31

In[111]:= (\* End of Symbolic computation \*)

In[112]:= (\* - End of Luttinger-Ward-Skeleton - Copyright © 2021 by Behnam Farid \*)
